# Supplementary material for: Guided Safe Shooting: model based reinforcement learning with safety constraints
Source: arXiv:2206.09743 source file (2024-09-12)
Supplement: Supplementary file 1 [file appendix_method.tex]

\section{Method}

As done by \cite{thomas2021safe}, we assume that there is a set of irrecoverable states $s \in S_{\text{irr}}$ that are not unsafe in themselves but that lead to unsafe states.
\paragraph{Assumption 1}
\label{ass1}
There exists a horizon $H^* \in \mathbf{N}$ for which, if the system is in an irrecoverable state $s \in S_{\text{irr}}$, any sequence of actions of length $h > H^*$ will lead to an unsafe state.

Divergent search methods, as \gls{me}, can discover, given enough iterations, all reachable behaviors starting from a state $s_i$.
The number of iterations is not an issue, thanks to performing them in a model, thus avoiding any unnecessary interaction with the real system.
If we assume that we start in $s_0 \notin S_{\text{irr}}$, the set of next possible states $s_1^i$ can contain only safe states and irrecoverable ones.
Thus, by planning in a good model for $H>H^*$ we can know which of the states $s_1^i$ are safe and which one are irrecoverable and only select the policies that lead us to safe states.
This permits our agent and model to always keep the system in safe states.

\Gadd{all the following section is a bit MEH....}

In practice, we never have a perfect model.
At the same time, it is also impossible to prevent unsafe situations without having some prior information on the setting we are working in. 
For this, we assume that a dataset $\mathbf{D}$ showing safe and unsafe transitions is given by the engineer allowing us to pretrain our model, similarly to what was done in \cite{thananjeyan2021recovery}.
The constraint violations necessary to generate this dataset happen under strict human supervision by the engineer, preventing uncontrolled and possibly dangerous situations.
Pretraining the model on this dataset allows to know with good probability if a state is safe or irrecoverable.

In this work, we generate this initial dataset on which the model is pretrained by applying to the system random action sequences. 
This produces lower quality pretraining data compared to the one possibly provided by an engineer, thus giving us a lower bound on the performances of our method.
\Gadd{MEH....}
