# Supplementary material for: Guided Safe Shooting: model based reinforcement learning with safety constraints
Source: arXiv:2206.09743 source file (2024-09-12)
Supplement: Supplementary file 2 [file appendix_pseudocode.tex]

\section{MAP-Elites}
\label{app:me}

In \glsfirst{me} the behavior space $\mathcal{B}$ is discretized through a grid with the algorithm trying to fill every cell of the grid \citep{mouret2015illuminating}.
\gls{me} starts by sampling the parameters $\phi \in \Phi$ of $M$ policies from a random distribution and evaluating them in the environment.
The behavior descriptor $b_i \in \mathcal{B}$ of a policy $\phi_i$ is then calculated from the sequence of states traversed by the system during the policy evaluation.
This descriptor is then assigned to the corresponding cell in the discretized behavior space.
If no other policy with the same behavior descriptor is discovered, $\phi_i$ is stored as part of the collection of policies $\mathcal{A}_{\text{ME}}$ returned by the method.
On the contrary, the algorithm only stores, in the collection, the policy with the highest reward among those with the same behavior descriptor.
This allows the gradual increase of the quality of the policies stored in $\mathcal{A}_{\text{ME}}$.
At this point, \gls{me} randomly samples a policy from the collection, and uses it to generate a new policy $\tilde\phi_i$ to evaluate.
The generation of $\tilde\phi_i$ is done by adding random noise to its parameters through a \emph{variation function}  $\mathbb{V}(\cdot)$.
The cycle repeats until the given evaluation budget $N$ is depleted.
The pseudo-code of \gls{me} is shown in Alg. \ref{alg:map_elites}.

\begin{algorithm}[H]
\caption{MAP-Elites}\label{alg:map_elites}
\textbf{INPUT:} 
real system $p_{\text{real}}$,
initial state $s_0$,
evaluation budget $N$, 
parameter space $\Phi$, 
discretized behavior space $\mathcal{B}$, 
variation function $\mathbb{V}(\cdot)$, 
number of initial policies $M$,
episode length $H$;\\
\textbf{RESULT:} collection of policies $\mathcal{A}_{\text{ME}}$;\\
$\mathcal{A}_{\text{ME}} = \emptyset$ 
\algorithmiccomment{Initialize empty collection}\\

$\Gamma \leftarrow \text{SAMPLE}(\Phi, M)$ 
\algorithmiccomment{Sample initial $M$ policies}\\

$R, C, \mathcal{T}_{real} = \text{ROLLOUT}(p_{\text{real}}, s_0, \phi_i, H), ~~ \forall \phi_i \in \Gamma$ 
\algorithmiccomment{Evaluate policies in the real system}\\

$b_i = f(\phi_i, \mathcal{T}^i_{real}), \quad \forall \phi_i \in \Gamma ~ \text{and} ~ \forall \mathcal{T}^i_{real} \in \mathcal{T}_{real}$
\algorithmiccomment{Calculate policies behavior descriptors}\\

$\mathcal{A}_{\text{ME}} \leftarrow \phi_i,  ~~ \forall\phi_i \in \Gamma$ 
\algorithmiccomment{Store policies in collection}\\

\While{$N$ not depleted}{
$\Gamma \leftlsquigarrow \text{SELECT}(\mathcal{A}_{\text{ME}}, K, \Phi)$ 
\algorithmiccomment{Select $K$ policies from collection}\\

$\Tilde\Gamma \leftlsquigarrow \mathbb{V}(\Gamma)$ 
\algorithmiccomment{Generate new policies}\\

$R, C, \mathcal{T}_{real} = \text{ROLLOUT}(p_{\text{real}}, s_0, \Tilde\phi_i, H), ~~ \forall \Tilde\phi_i \in \Tilde\Gamma$ 
\algorithmiccomment{Evaluate new policies in the real system}\\

$b_i = f(\Tilde\phi_i, \mathcal{T}^i_{real}), \quad \forall \Tilde\phi_i \in \Tilde\Gamma ~ \text{and} ~ \forall \mathcal{T}^i_{real} \in \mathcal{T}_{real}$ 
\algorithmiccomment{Calculate behavior descriptors}\\

$\mathcal{A}_{\text{ME}} \leftarrow \Tilde\phi_i,  ~~ \forall\Tilde\phi_i \in \Tilde\Gamma$ 
\algorithmiccomment{Store policies in collection}\\
}
\end{algorithm}
\newpage 

\section{Planners Pseudocode}
This appendix contains the pseudo code of the three planners introduced in the paper.
Each planner evaluates a policy on the model through a ROLLOUT function detailed in Alg. \ref{alg:rollout}.

\begin{algorithm}[H]
\caption{ROLLOUT}
\label{alg:rollout}

\textbf{INPUT:} model $p$, initial state $s_0$, policy $\phi$, horizon length $h$;\\
\textbf{RESULT:} collected reward $R$, collected cost $C$, simulated trace $\mathcal{T}_{model}$;\\

$\mathcal{T}_{model} = \emptyset$ \algorithmiccomment{Initialize empty trace}\\
\For{j in [0, \dots, h]}{
$a_{j} \leftlsquigarrow \phi(s_{j})$ \algorithmiccomment{Draw action from policy}\\
$s_{j+1} \leftlsquigarrow p(s_{j}, a_{j})$\algorithmiccomment{Draw next predicted state}\\
$\mathcal{T}_{model} = \mathcal{T}_{model} \bigcup (s_{j}, a_{j})$ \algorithmiccomment{Update trace}\\
}
$R = \sum_{j=0}^{h} \gamma^j r(s_{j}, a_{j})$ \algorithmiccomment{Calculate reward of action sequence}\\
$C = \sum_{j=0}^{h} \gamma^j c(s_{j}, a_{j})$ \algorithmiccomment{Calculate cost of action sequence}\\
\end{algorithm}

\subsection{Safe Random Shooting}
\label{app:rs}
Algorithm \ref{alg:rss} shows the pseudocode of the \glsfirst{rss} planner.

\begin{algorithm}[H]
\caption{\gls{rss}}
\label{alg:rss}
\textbf{INPUT:} model $p$, current real-system state $s_t$, planning horizon $h$, evaluated action sequences $N$, action space $\mathcal{A}$;\\
\textbf{RESULT:} action to perform $a_t$;\\
$\text{AS} = \emptyset$ \algorithmiccomment{Initialize empty collection of action sequences}\\
\For{i in [0, \dots, N]}{
    $\phi_i = [a_t, \dots, a_{t+h}] \leftlsquigarrow \text{SAMPLE}(\mathcal{A}, h)$ \algorithmiccomment{Sample action sequence}\\
    $R_i$, $C_i$, $\mathcal{T}^i_{model}$ = ROLLOUT($p$, $s_t$, $\phi_i$, $h$) \algorithmiccomment{Evaluate action sequence}\\
    $\text{AS} = \text{AS} \bigcup (\phi_i, R_i, C_i)$ \algorithmiccomment{Store evaluated  action sequence}\\
}
$\text{AS}_{\text{lc}} \leftlsquigarrow \text{AS}$ \algorithmiccomment{Get action sequences with lowest cost}\\
$\phi_{\text{best}} \leftlsquigarrow \text{AS}_{\text{lc}}$ \algorithmiccomment{Get action sequence with highest reward}\\
$a_t \leftlsquigarrow \phi_{\text{best}}(s_t)$\algorithmiccomment{Get next action}\\
\end{algorithm}

\subsection{Safe MAP-Elites}
\label{app:mes}
Algorithm \ref{alg:mes} shows the pseudocode of the \glsfirst{mes} method.
The SELECT function is shown in Alg. \ref{alg:mes_select}.

\begin{algorithm}[H]
\caption{SELECT function of \gls{mes} planner}
\label{alg:mes_select}
\textbf{INPUT:} 
Collection of policies $\mathcal{A}_{\text{ME}}$,
Number of policies to select $K$,
Policy parameter space $\Phi$
;\\
\textbf{RESULT:} set of selected policies $\Gamma$;\\
$\Gamma = \emptyset$ 
\algorithmiccomment{Initialize empty set of selected policies}\\

$\Gamma \leftlsquigarrow \mathcal{A}_{\text{ME}}[C=0]$
\algorithmiccomment{Select policies with $C=0$ from collection}\

\If{$\text{size}(\Gamma) < K$}{
$\Gamma = \Gamma \bigcup \text{SAMPLE}(\Phi)$ 
\algorithmiccomment{Sample missing policies from parameter space}\\
}
\end{algorithm}

\begin{algorithm}[H]
\caption{\gls{mes}}
\label{alg:mes}
\textbf{INPUT:} 
model $p$, 
current real-system state $s_t$, 
planning horizon $h$, 
evaluated action sequences $N$, 
discretized behavior space $\mathcal{B}$,
variation function $\mathbb{V}(\cdot)$,
number of initial policies $M$,
number of policies per iteration $K$,
policy parameter space $\Phi$
;\\
\textbf{RESULT:} action to perform $a_t$;\\
$\mathcal{A}_{\text{ME}} = \emptyset$ 
\algorithmiccomment{Initialize empty collection of policies}\\

$\Gamma \leftarrow \text{SAMPLE}(\Phi, M)$ 
\algorithmiccomment{Sample initial $M$ policies}\\

$R, C, \mathcal{T}_{model} = \text{ROLLOUT}(p, s_t, \phi_i, h), \quad \forall \phi_i \in \Gamma$ 
\algorithmiccomment{Evaluate policies in the model}\\

$b_i = f(\phi_i, \mathcal{T}^i_{model}), \quad \forall \phi_i \in \Gamma ~ \text{and} ~ \forall \mathcal{T}^i_{model} \in \mathcal{T}_{model}$
\algorithmiccomment{Calculate policies behavior descriptors}\\

$\mathcal{A}_{\text{ME}} \leftarrow \phi_i,  ~~ \forall\phi_i \in \Gamma$ 
\algorithmiccomment{Store policies in collection}\\

\While{$N$ not depleted}{
$\Gamma \leftlsquigarrow \text{SELECT}(\mathcal{A}_{\text{ME}}, K, \Phi)$ 
\algorithmiccomment{Select $K$ policies with $C=0$ from collection}\\

$\Tilde\Gamma \leftlsquigarrow \mathbb{V}(\Gamma)$ 
\algorithmiccomment{Generate new policies}\\

$R, C, \mathcal{T}_{model} = \text{ROLLOUT}(p, s_t, \Tilde\phi_i, h), \quad \forall \Tilde\phi_i \in \Tilde\Gamma$ 
\algorithmiccomment{Evaluate new policies in the model}\\

$b_i = f(\Tilde\phi_i, \mathcal{T}^i_{model}), \quad \forall \Tilde\phi_i \in \Tilde\Gamma ~ \text{and} ~ \forall \mathcal{T}^i_{model} \in \mathcal{T}_{model}$ 
\algorithmiccomment{Calculate behavior descriptors}\\

$\mathcal{A}_{\text{ME}} \leftarrow \Tilde\phi_i,  ~~ \forall\Tilde\phi_i \in \Tilde\Gamma$ 
\algorithmiccomment{Store policies in collection}\\
}

$\Gamma_{\text{lc}} \leftlsquigarrow \text{AS}$ 
\algorithmiccomment{Get policies with lowest cost}\\

$\phi_{\text{best}} \leftlsquigarrow \Gamma_{\text{lc}}$ 
\algorithmiccomment{Get policy with highest reward}\\

$a_t \leftlsquigarrow \phi_{\text{best}}(s_t)$
\algorithmiccomment{Get next action}\\
\end{algorithm}

\subsection{Pareto Safe MAP-Elites}
\label{app:mesp}
The \glsfirst{mesp} planner works similarly to the \gls{mes} one with the exception of the SELECT function at line 9 of Alg. \ref{alg:mes}.
So for this planner we just report the pseudocode of this function in Alg. \ref{alg:mesp_select}.

\begin{algorithm}[H]
\caption{SELECT function of \gls{mesp} planner}
\label{alg:mesp_select}
\textbf{INPUT:} 
Collection of policies $\mathcal{A}_{\text{ME}}$,
Number of policies to select $K$,
Policy parameter space $\Phi$
;\\
\textbf{RESULT:} set of selected policies $\Gamma$;\\
$\Gamma = \emptyset$ 
\algorithmiccomment{Initialize empty set of selected policies}\\

$[\Gamma^0_{\text{ND}}, \dots, \Gamma^n_{\text{ND}}] \leftlsquigarrow $ NON\_DOMINATED\_SORT($\mathcal{A}_{\text{ME}}$)
\algorithmiccomment{Sort collection into non dominated fronts}\\

$i = 0$\\
\While{size$(\Gamma) < K$}{
$\Gamma \leftlsquigarrow \Gamma^i_{\text{ND}}$
\algorithmiccomment{Select policies from best front}\\
$i = i+1$\\
}
\end{algorithm}
\newpage
