# Supplementary material for: Guided Safe Shooting: model based reinforcement learning with safety constraints
Source: arXiv:2206.09743 source file (2024-09-12)
Supplement: Supplementary file 3 [file appendix.tex]

\documentclass{article}
\usepackage[final]{neurips_2023}

\usepackage[ruled, noend]{algorithm2e}
\usepackage{notations}
\usepackage{caption}
\captionsetup{singlelinecheck=off}

\usepackage[utf8]{inputenc} % allow utf-8 input
\usepackage[T1]{fontenc}    % use 8-bit T1 fonts
\usepackage{url}            % simple URL typesetting
\usepackage{booktabs}       % professional-quality tables
\usepackage{subfiles}
\usepackage{amsfonts}       % blackboard math symbols
\usepackage{nicefrac}       % compact symbols for 1/2, etc.
\usepackage{microtype}      % microtypography

\usepackage[pdftex]{graphicx}
\usepackage[acronym]{glossaries}
\usepackage{enumitem}
\usepackage{lipsum}  
\usepackage{amsmath, MnSymbol}
\usepackage{wrapfig}
\usepackage{float}
\usepackage{MnSymbol}
\usepackage{subfig}

\usepackage{xcolor}
\definecolor{darkblue}{rgb}{0,0,0.5}
\definecolor{firebrick}{rgb}{0.75,0.125,0.125}
\definecolor{darkgreen}{rgb}{0,0.5,0}
\definecolor{light-gray}{gray}{0.5}

\usepackage[colorlinks=true,linkcolor=firebrick,citecolor=darkgreen,urlcolor=darkblue]{hyperref}

\author{}
% Neurips Title
\title{Supplementary materials}
\begin{document}

\maketitle
\input{sections/appendix_environments}
\input{sections/appendix_plots}
\include{sections/appendix_metrics}
\input{sections/appendix_hyperparams}

\end{document}
