# Supplementary material for: Guided Safe Shooting: model based reinforcement learning with safety constraints
Source: arXiv:2206.09743 source file (2024-09-12)
Supplement: Supplementary file 4 [file appendix_video.tex]

\section{Videos}
